# Supplementary material for: Liquid film rupture beyond the thin-film equation: a multi-component lattice Boltzmann study
Source: arXiv:2203.13717 ancillary file (2022-06-16)
Supplement: Supplementary file 1 [file supplementary.pdf]

# Supplementary Information for "Liquid film rupture beyond the thin-film equation: a multi-component lattice Boltzmann study"

**Francesca Pelusi**
Helmholtz Institute Erlangen-Nürnberg for Renewable Energy (IEK-11), Forschungszentrum Jülich GmbH
Cauerstraße 1, 91058 Erlangen, Germany
f.pelusi@fz-juelich.de

**Marcello Sega**
Helmholtz Institute Erlangen-Nürnberg for Renewable Energy (IEK-11), Forschungszentrum Jülich GmbH
Cauerstraße 1, 91058 Erlangen, Germany

**Jens Harting**
Helmholtz Institute Erlangen-Nürnberg for Renewable Energy (IEK-11), Forschungszentrum Jülich GmbH
Cauerstraße 1, 91058 Erlangen, Germany
Department of Chemical and Biological Engineering and Department of Physics
Friedrich-Alexander-Universität Erlangen-Nüremberg
Cauerstraße 1, 91058 Erlangen, Germany

# 1 Phase diagram, surface tension and interface width

As mentioned in Section II of the main text, a dedicated phase-separation experiment is needed in order to get the most suitable range of the coupling parameter $G_{AB}$ in relation to the choice of the initial bulk densities $\rho_A$ and $\rho_B$. In this kind of experiment, one half of the domain is occupied with the majority of the first $A$, and the second half with the component $B$. When the system reaches its equilibrium configuration, the maximum and minimum density values of component $A$ are measured as a function of $G_{AB}$, as shown in Fig. S2(a). This experiment allows measuring also the interface width at varying the coupling parameter (see Fig. S2(b)).

Furthermore, a Laplace experiment allows to measure the surface tension $\gamma$ (see Fig. S2(b)).

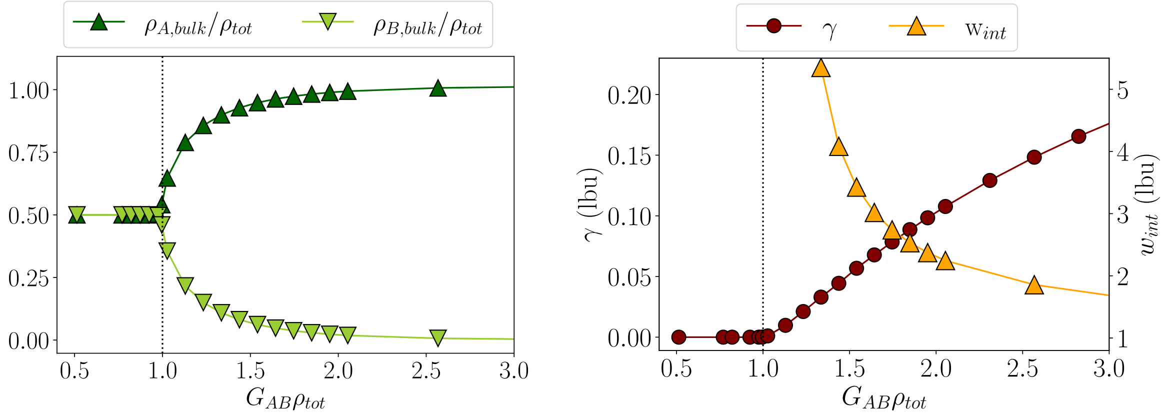


(a) (b)

Fig.S 1: Panel (a): a measurement of the minimum and maximum bulk densities for component $A$ in a phase-segregation experiments. Data are shown as a function of the strength intensity $G_{AB}$, normalised to the total density $\rho_{tot} = \rho_A + \rho_B$, with $\rho_A$ and $\rho_B$ the initial bulk densities (see the main text for further details). Panel (b): interface width $w_{int}$ and surface tension $\gamma$ as a function of $G_{AB}/\rho_{tot}$. $\gamma$ is measured via a dedicated Laplace experiment. Vertical dashed lines correspond to the critical point.

# 2 Power spectra

In Fig.5 of the main text we show the power spectra $S(q,t)$, normalised to the initial value $S(q,0)$, as a function of $q$. These data are taken at three different times $t_1$, $t_2$ and $t_3$, which are different for each panel: $t_1$ corresponds to an early time after the perturbation, $t_3$ is a time close to the rupture time, and $t_2$ an intermediate time. The values of these times (given in lbu) are reported in Table 1.

| $h_0$ (lbu) | $\theta_{eq}$ (°) | $t_1$ (lbu) | $t_2$ (lbu) | $t_3$ (lbu) |
|---|---|---|---|---|
| 6 | 180 | $4\ 10^2$ | $7\ 10^2$ | $10^3$ |
| 6 | 130 | $3\ 10^3$ | $7\ 10^3$ | $1.1\ 10^4$ |
| 6 | 90 | $1.1\ 10^4$ | $1.7\ 10^4$ | $2.1\ 10^4$ |
| 7 | 180 | $3\ 10^3$ | $6\ 10^3$ | $9\ 10^3$ |
| 7 | 130 | $9\ 10^3$ | $2.5\ 10^4$ | $3.8\ 10^4$ |
| 7 | 90 | $3.6\ 10^4$ | $5\ 10^4$ | $6.2\ 10^4$ |
| 8 | 180 | $4\ 10^3$ | $1.2\ 10^4$ | $2\ 10^4$ |
| 8 | 130 | $10^4$ | $2.7\ 10^4$ | $4\ 10^4$ |
| 8 | 90 | $3\ 10^4$ | $5\ 10^4$ | $8\ 10^4$ |

Table S 1: Values of $t_1$, $t_2$ and $t_3$ for the data shown in Fig.5 of the main text.
